# Supplementary material for: HDR-Polar1K: An HDR Stokes Image Dataset for Learning Color-Polarization Reconstruction
Source: arXiv:2611.35068 source file (2026-11-25)
Supplement: Supplementary file 1 [file supp-real-metadata-regions.tex]

\newcommand{\foliagemarks}{%
\markregion{49.7092}{23.8137}{1.8301}{yellow}%
\markregion{20.8399}{1.5098}{1.8301}{cyan}%
}
